# Supplementary material for: Authenticity and exclusion: social media algorithms and the dynamics of belonging in epistemic communities
Source: arXiv:2407.08552 source file (2024-10-21)
Supplement: Supplementary file 1 [file appendix.tex]

\section{Additional experiments}

\subsection{Variations of minority group shares}
\label{app_sec:4.2}
% Results of variations in minority group size, graph structure and rec policy
Figure~\ref{fig:size_real_graph_ratio_rec_0} explores variations of the experiment with different minority group shares. We find that, as long as the minority group is small, both the decreased visibility for professional content by the minority group and amplification thereof persist.
Similar effects emerge when assuming fully connected and random graph structures rather than the homophilic case considered previously.
This gives further evidence to our explanation of the real graph policy as culprit for the amplification effect.
In fact, Figures~\ref{fig:random_ratio_rec_0} and \ref{fig:topic_ratio_rec_0} depict analogous results for random and topic match recommendation policies showing that the amplification effect dissipates under these policies. While professional content has equal visibility for minority and majority group members in random and fully connected graph structures, a homophilic graph structure translates to an approximately constant disadvantage for minority group visibility with random recommendation policy.

Our findings indicate that a homophilic graph structure reduces the visibility of professional content for minority groups. This disadvantage is further perpetuated and amplified by recommendation algorithms, such as the real graph policy, which rely on historical interaction counts.

\begin{figure}[H]
    \centering
    \includegraphics[scale=0.6]{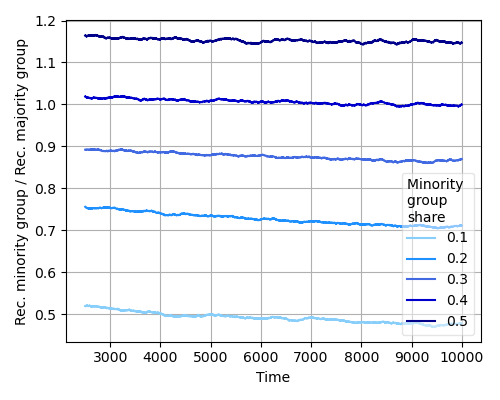}
    \caption{Moving average (window size = 1,000) of ratio of average professional content recommendations for content created by minority and majority groups. Data obtained from 10 simulation runs for each minority group share value, using \textbf{real graph recommendation policy and homophilic network structure}.}
    \label{fig:size_real_graph_ratio_rec_0}
\end{figure}

%Moving average (window size = 1,000) of ratio of the aver-
%age number of recommendations for professional topic content created by minority and majority group users over time

\begin{figure}[H]
    \centering
    \includegraphics[scale=0.6]{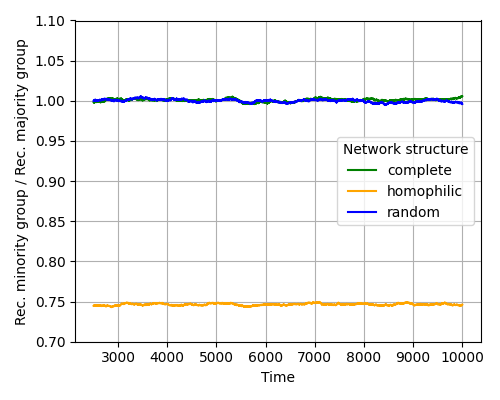}
    \caption{Moving average (window size = 1,000) of ratio of the average number of recommendations for professional topic content created by minority and majority group users over time, using \textbf{random recommendation policy}. Results are averaged over 20 simulation runs.}
    \label{fig:random_ratio_rec_0}
\end{figure}

\begin{figure}[H]
    \centering
    \includegraphics[scale=0.6]{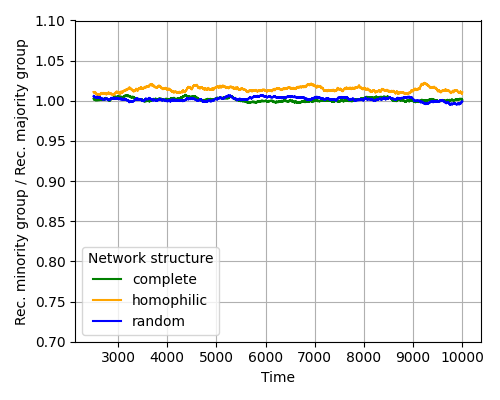}
    \caption{Moving average (window size = 1,000) of ratio of the average number of recommendations for professional topic content created by minority and majority group users over time, using \textbf{topic match recommendation policy}. Results are averaged over 20 simulation runs.}
    \label{fig:topic_ratio_rec_0}
\end{figure}

\section{Variations of graph structure} %p
The base case of the experiments discussed in Section~\ref{sec:results} assumes a homophilic network structure created by a stochastic block model, i.e. directed edges between users in the graph are formed by throwing coins with probabilities $p=(p^{\text{edge}}_{\text{maj-maj}}, p^{\text{edge}}_{\text{min-min}}, p^{\text{edge}}_{\text{maj-min}}, p^{\text{edge}}_{\text{min-maj}})$. Here, the subscript describes the groups of the user pair an edge is sampled for.
We use the parameter choices $p=(0.5,0.4,0.1,0.1)$ in the main experiments to reflect a realistic scenario. However, we also explore different parameter configurations to assess the robustness of our findings.

Figure~\ref{fig:p_real_graph} depicts the ratio of the average number of recommendations
for professional topic content created by minority and majority group users over time with real graph recommendation policy for various stochastic block model parameters. As before, we observe that professional content created by the minority group is promoted less frequently than comparable content created by the majority group. This disadvantage is reinforced and exacerbated by the real graph recommendation algorithm which relies on historical interaction counts.
Notably these observations are still true when the network structure is balanced with $p=(0.5,0.5,0.5,0.5)$ which corresponds to the random network structure displayed in Figure~\ref{fig:real_graph_ratio_rec_0}.

\begin{figure}[H]
    \centering
    \includegraphics[scale=0.6]{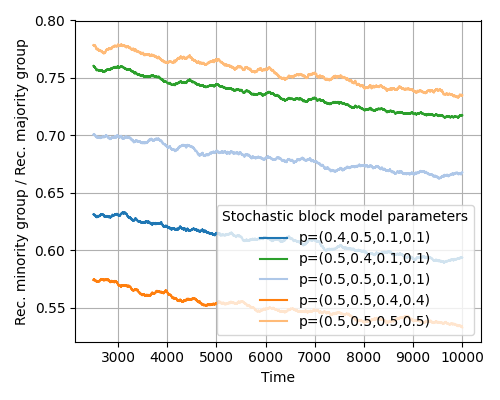}
    \caption{Moving average (window size = 1,000) of ratio of the average number of recommendations for professional topic content created by minority and majority group users over time, using \textbf{real graph recommendation policy and homophilic networks with different stochastic block model parameters}. Results are averaged over 10 simulation runs.}
    \label{fig:p_real_graph}
\end{figure}

\section{Variations of interaction model} %b
The real graph recommendation policy draws on an interaction function with four parameters: $\beta_1$ for the number of common outgoing edges, $\beta_2$ for the number of common incoming edges, $\beta_3$ for the a distance metric, and $\beta_4$ for the interaction count between users. For the simulations described in the main text, we assume a parameter vector $\beta=(1,1,-1,5)$ to specifically study the impact of the interaction count feature. Here, we explore other parameter choices for robustness. 

Figure~\ref{fig:b_real_graph} depicts the ratio of the average number of recommendations for the professional topic content created by the minority and majority groups for various parameter vector choices. We specifically vary $\beta_4$, i.e. the parameter corresponding to the interaction count feature, between 1 and 10 in increments of 1. We can see that professional content created by the minority group is recommended less frequently than content recommended by the majority group over all parameter variations. In most cases, there is an amplification effect over time leading to more and more disadvantage for the minority group. Yet, this is not the case for $\beta=(1,1,-1,1)$ in which case majority group created professional content is increasing in recommendation ratio over time. This finding showcases the importance of the interaction count feature in the tie strength model. As long as the importance of the tie strength features outweighs other features, minority group created professional content is less and less recommended relative to the majority group created professional content over time.

\begin{figure}[H]
    \centering
    \includegraphics[scale=0.6]{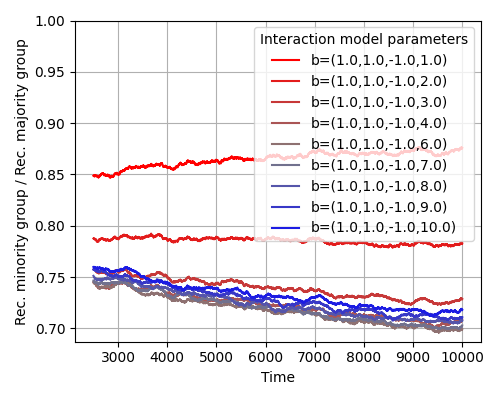}
    \caption{Moving average (window size = 1,000) of ratio of the average number of recommendations for professional topic content created by minority and majority group users over time, using \textbf{real graph recommendation policy and interaction models with different parameters}. Results are averaged over 10 simulation runs.}
    \label{fig:b_real_graph}
\end{figure}

\section{Supplementary figures}
\label{app:supp_fig}

\begin{figure}[H]
    \centering
    \includegraphics[scale=0.6]{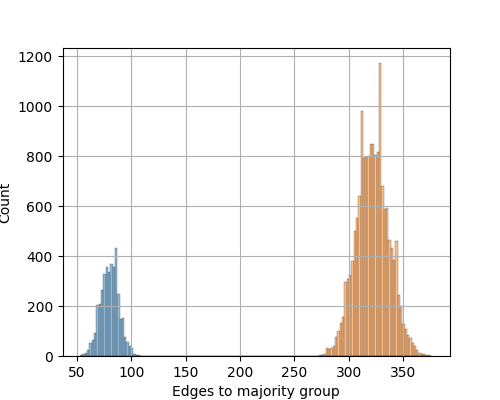}
    \includegraphics[scale=0.6]{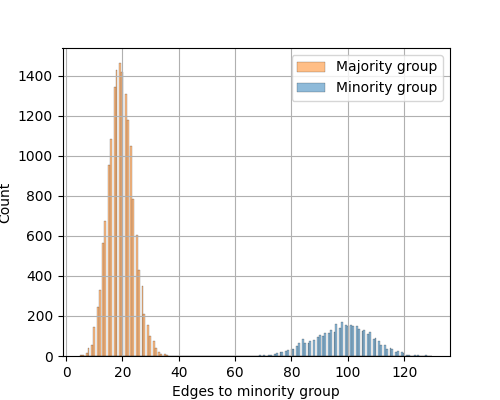}
    \caption{Histogram of the number of outgoing edges (i.e. `follow' relationships) to majority and minority group users over 20 simulation runs. On average, both groups have more in-group connections than connections across groups.}
    \label{fig:edge_hist}
\end{figure}

\begin{figure}[H]
    \centering
    \includegraphics[scale=0.6]{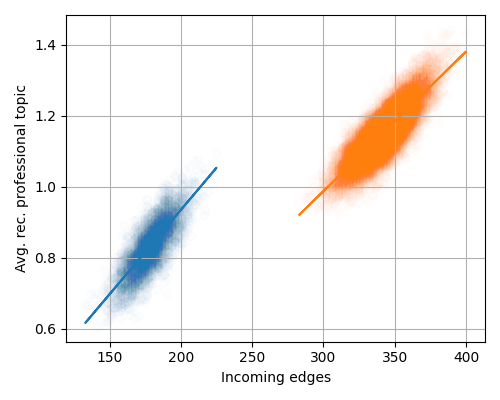}
    \includegraphics[scale=0.6]{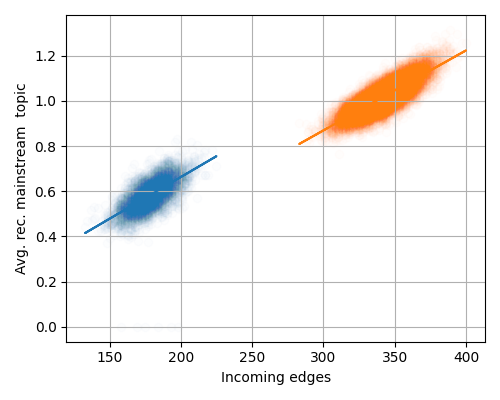}
    \includegraphics[scale=0.6]{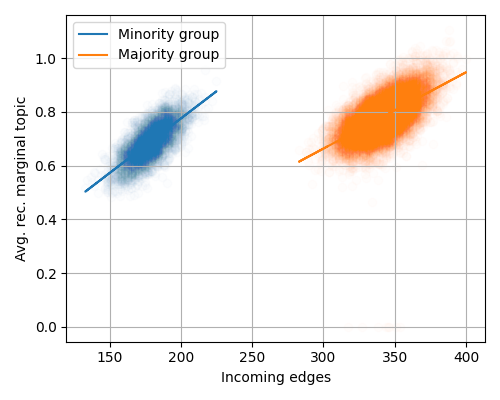}
    \caption{Average number of recommendations and incoming edges by content topic and creator group with linear approximations. Each point corresponds to one user in one of 20 simulation run with \textbf{homophilic network and real graph recommendation policy}.} \label{fig:size_real_graph_homophilic_incoming_edges_rec}
\end{figure}
